# Supplementary material for: Optimal Active Fault Detection in Inverter-Based Grids
Source: arXiv:2209.06760 source file (2022-09-14)
Supplement: Supplementary file 1 [file Appendix.tex]

\begin{appendix}
bsdfh

\end{appendix}
